# Supplementary material for: Heavy Fermion Quantum Criticality and Destruction of the Kondo Effect in a Nickel Oxypnictide
Source: arXiv:1408.3132 source file (2014-08-13)
Supplement: Supplementary file 1 [file CeNiAsO_pressure_140416__NM_SI.pdf]

## *Supplementary Information for:*

# Heavy Fermion Quantum Criticality and Destruction of the Kondo Effect in a Nickel Oxypnictide

Yongkang Luo[1,2], Leonid Pourovskii[3,4], Stephen Rowley[2], Yuke Li[5,1], Chunmu Feng[1], Antoine Georges[3], Jianhui Dai[5,1], Guanghan Cao[1], Zhu'an Xu[1*], Qimiao Si[6], and N. P. Ong[2]

[1]*Department of Physics and State Key Laboratory of Silicon Materials, Zhejiang University, Hangzhou 310027, P. R. China,*

[2]*Department of Physics, Princeton University, Princeton, New Jersey 08544, U.S.A,*

[3]*Centre de Physique Théorique, École Polytechnique, CNRS, 91128 Palaiseau Cedex, France,*

[4]*Swedish e-science Research Centre (SeRC), Department of Physics, Chemistry and Biology (IFM), Linköping University, Linköping, Sweden*

[5]*Department of Physics, Hangzhou Normal University, Hangzhou 310036, P. R. China, and*

[6]*Department of Physics and Astronomy, Rice University, Houston, TX 77005, USA*

(Dated: April 16, 2014)

* Electronic address: zhuan@zju.edu.cn

### *SI I: Additional evidences for quantum critical point.*

In Figure S1a we show the temperature-derivative of the resistivity, $d\rho/dT$, as a function of temperature in the vicinity of the critical pressure $p_c$=6.5 kbar. For the case of $p$=5.3 kbar which is lower than $p_c$, a pronounced peak is seen, which is a sign of the AFM phase transition. As pressure is increased towards $p_c$, the peak position shifts to lower temperature, and the height of the peak also shrinks. For $p$=6.7 kbar, the peak is very weak and broad, indicating nearly liner $\rho$ vs. $T$ correlation ($n$∼1, see Figure S1b). When pressure is further increased, the center position of this broad peak moves towards higher temperature, and linear $d\rho/dT$ vs. $T$ correlation was seen in the up-moving of the peak, which is a characteristic of Fermi-liquid (FL) behavior ($n$∼2). This broad peak should be associated with the occurrence of Kondo coherence. The $d\rho/dT$ peak of cross-over type due to coherent Kondo scattering above $p_c$ differs in shape from that of the AFM transition below $p_c$; this adds additional evidence that the magnetic ordering of Ce ions has been totally suppressed at $p_c$ and it evolves into a Kondo lattice FL-like metal.

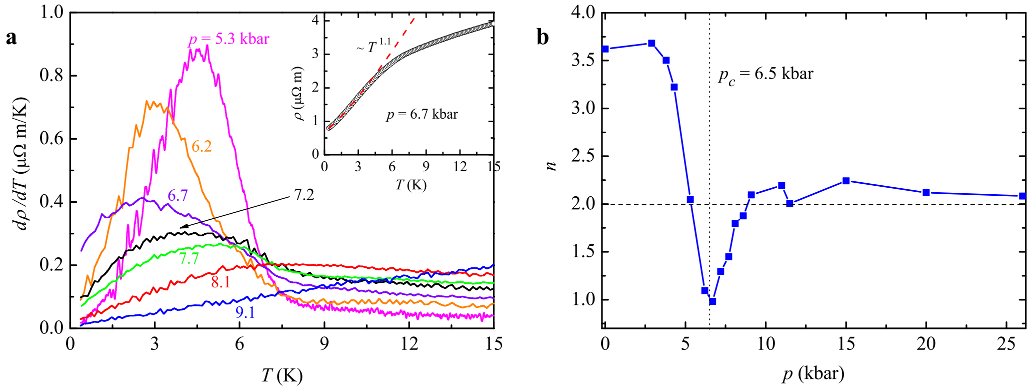


**Figure S1 | Further information from $\rho(T)$ profiles. a**, When $p<p_c$, $d\rho/dT$ shows a sharp peak at the AFM transition temperature. For $p>p_c$, the peak broadens, and should be attributed to be the coherent Kondo scattering as discussed in the context. **b**, pressure dependence of the resistivity exponent $n$, derived from $\rho(T)$ at $T\leq5$ K.

To get a more clear picture of the pressure dependence of the exponent of the power law in $\rho(T)$, we show $n$ as a function of pressure in Figure S1b. All the $\rho(T)$ curves were fit

to $\rho(T)=\rho_0+AT^n$, and the fitting region was fixed as $0<T\leq5$ K. The derived $n(p)$ shows a clear dip and is close to 1 at around $p_c$=6.5 kbar, strongly manifesting the non-FL behavior. For $p>p_c$, $n$ elevates and keeps in $1.8\leq n\leq$ 2.2, which is a typical signature of a FL metal. Such $n(p)$ is consistent with the local-fitting result shown in Figure 2a, and thus provides additional evidence for the unique quantum critical point.

## *SI II: Structural characterizations by X-ray diffractions*

Samples of $CeNiAs_{1-x}P_xO$ were characterized by the powder X-ray differaction (XRD). All the XRD peaks can be well indexed based on the tetragonal ZrCuSiAs-type structure with the space group P4/$nmm$ (No.129), and the lattice parameters $a$ and $c$ were calculated from the least square fit on at least 25 peaks on XRD patterns. Very little impurity phases can be detected, as marked by the labels "*". Most likely, the impurity is $Ce_2O_3$, which shows a 5.7 K-AFM-transition[1] that might result in an magnetic anomaly in specific heat (Figure 3) and divergence in magnetic susceptibility in zero temperature limit (Figure 4). As shown in Figure S2, the XRD peaks shift toward righthand, especially for the high angle reflections.

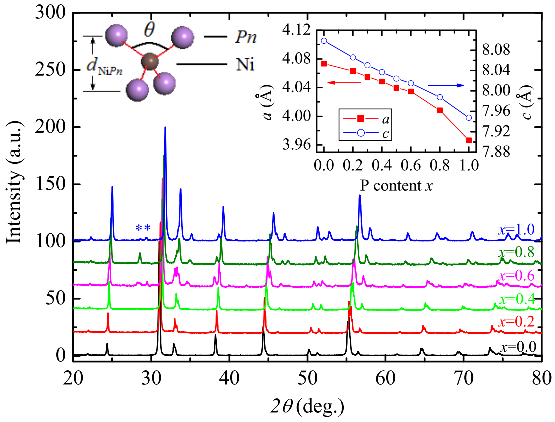


**Figure S2 | Structural characterization by XRD for $CeNiAs_{1-x}P_xO$.** Main frame, XRD patterns of $x$=0, 0.2, 0.4, 0.6, 0.8 and 1.0 samples measured at room temperature. "*" marks the possible impurity phase of $Ce_2O_3$. The insets display the sketch of the Ni$Pn$ layer, as well as the lattice parameters $a$ and $c$ as functions of P doping content $x$.

**Table S1: Comparison of lattice parameters between CeNiAsO and CeNiPO.** Results from Rietveld refinement. Atomic positions: Ce (1/4, 1/4, $z_{\mathrm{Ce}}$), Ni (3/4, 1/4, 1/2), $Pn$ (1/4, 1/4, $z_{Pn}$), O (3/4, 1/4, 0).

| CeNi$Pn$O | CeNiAsO | CeNiPO |
|---|---|---|
| $a$ (Å) | 4.0767 | 3.9652 |
| $c$ (Å) | 8.1015 | 7.9526 |
| $z_{\mathrm{Ce}}$ | 0.1465 | 0.1560 |
| $z_{Pn}$ | 0.6434 | 0.6322 |
| $d_{\mathrm{Ni}Pn}$ (Å) | 2.3235 | 2.1027 |
| $\theta_{Pn-\mathrm{Ni}-Pn}$ (°) | 120.6 | 124.1 |
| $R_{wp}$ | 8.11% | 12.39% |
| $R_p$ | 5.73% | 9.20% |
| $S$ | 0.88 | 1.25 |

This observation is consistent with the lattice parameter calculation results shown in the inset of Figure S2. We also performed the Rietveld refinement[2] on the two end compounds, CeNiAsO and CeNiPO. The remarkable differences are listed in Table S1. This structural feature supports the increasing Kondo coupling between Ni-3$d$ and Ce-4$f$ electrons, as discussed in the main article.

### *SI III: Resistivity and phase diagram of CeNiAs$_{1-x}$P$_x$O*

The transport properties of CeNiAs$_{1-x}$P$_x$O are displayed in Figure S3. One can find that in those P/As-doped samples, the resistivities at room temperature, i.e. $\rho$(300K), are relatively larger than the parent compounds CeNiAsO and CeNiPO. We attributed this to the disorder/impurity scattering brought in by P/As substitution. To see the intrinsic chemical pressure effect of CeNiAs$_{1-x}$P$_x$O, we fit the $\rho(T)$ to the formula $\rho$=$\rho_0$+$\Delta\rho$, in which the residual resistivity $\rho_0$ here is contributed by disorder/impurity scattering, as well

as the spin fluctuation if near the QCP as mentioned in the main article. Similar to the pressurized case, the two antiferromagnetic (AFM) transitions, noted by $T_{N1}$ and $T_{N2}$ are suppressed (Figure S3c-d), and the $\rho(T)$ profile evolves into FL behavior in the heavily P-doped samples (Figure S3b), while non-FL-like $\rho(T)$ dependence is observed around the critical point $x_c$=0.4.

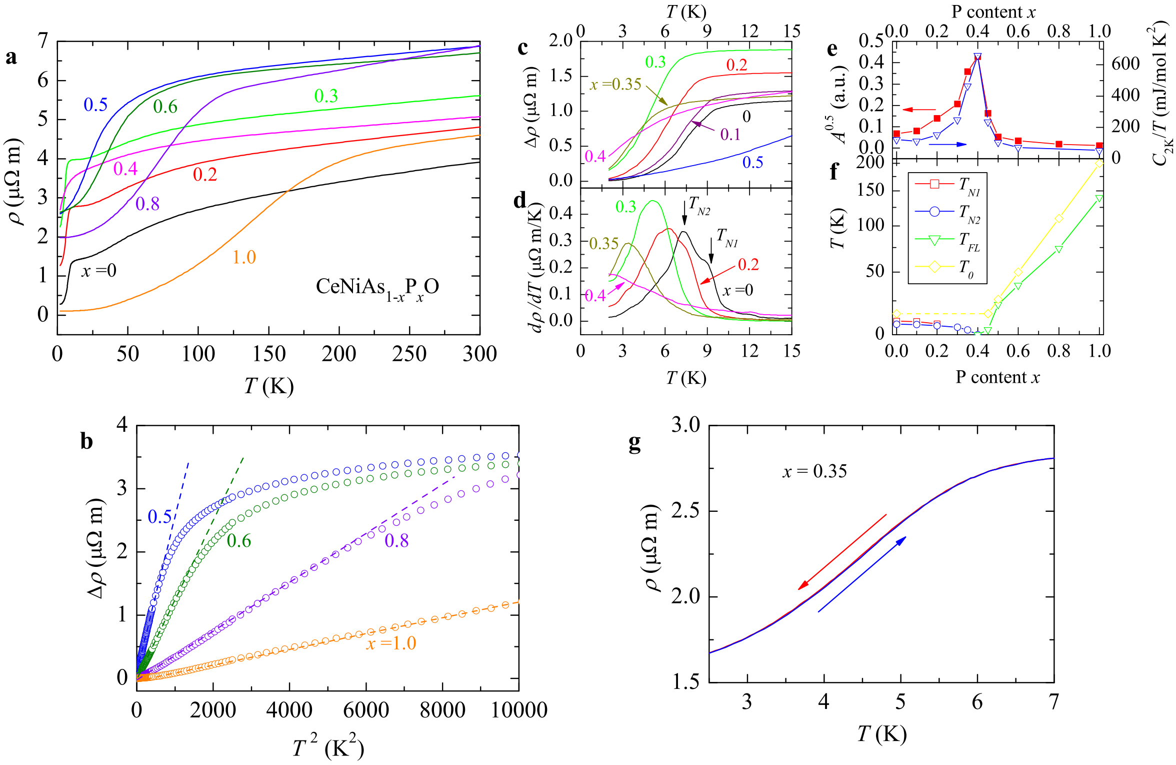


**Figure S3 | Resistivity of CeNiAs$_{1-x}$P$_x$O.** **a**, temperature dependence of resistivity $\rho(T)$ of CeNiAs$_{1-x}$P$_x$O. **b**, $\Delta\rho$ in the $T^2$ plot. **c**, enlarged plot of $\Delta\rho(T)$ in the low temperature region. **d**, derivative resistivity $d\rho/dT$ as a function of temperature. **e**, the $A^{0.5}$ coefficient and $C^{2K}/T$ as functions of P content $x$. **f**, a schematic phase diagram of CeNiAs$_{1-x}$P$_x$O. **g**, a resistivity thermal cycle measurement on CeNiAs$_{0.65}$P$_{0.35}$O, the red curve taken when cooling down while the blue one taken when warming up.

Furthermore, we can see the increasing Kondo coupling which is characterized by the hump in the $\rho(T)$ curves. For CeNiPO, the $T^2$-law of $\rho$ extends to up to 140 K. We also fit

the $\Delta\rho(T)$ to the formula $\Delta\rho(T)=AT^n$, where the square root of $A$ coefficient is plotted in Figure S3e, together with the specific heat $C^{2K}/T$ measured at 2 K. The peaks in $\rho_0$ (data not shown), $A^{0.5}$, $C^{2K}/T$ support the picture of heavy fermion quantum critical point around $x_c$=0.4. A simplified phase diagram is given in Figure S3f. In general, the effect of P doping in CeNiAsO is very similar to that of the hydrostatic pressure. We should, however, note that the chemical pressure effect in the 100% P end, CeNiPO, is considerably more pronounced than the highest hydrostatic pressure case 26 kbar. For instance, in CeNiPO, $T_{FL}\sim$140 K and $T_0\sim$200 K, which are much higher than the corresponding values obtained at $p$=26 kbar. Roughly estimated, at least 50 kbar of external pressure should be applied on CeNiAsO to get a comparable pressure effect as in CeNiPO. We also took the resistivity thermal cycle measurement on $CeNiAs_{0.65}P_{0.35}O$ which is thought to be close to the quantum phase transition. As is shown in Figure S3g, the red curve stands for the data collected when the sample was cooling down, while the blue one was collected in the warming up process. It can be seen that, the two curves overlaps so well that thermal hysteresis is hardly seen. This strongly confirms that $CeNiAs_{1-x}P_x$ keeps the 2nd order feature of a phase transition when it is close to $x_c$.

## *SI IV: Isothermal magnetization and Hall coefficient of* $CeNiAs_{1-x}P_xO$

$M(H)$ curve reflects the spin polarization driven by an external magnetic field. In the case of $Ce^{3+}$ in a local tetragonal crystalline electric field surrounding where $\Gamma_6$ doublet ($|\pm 1/2\rangle$ ) was suggested to be the ground state [3], the expected saturated $M$ is about 1 $\mu_B$ in a polycrystalline sample, which was seen in $CeFeAs_{1-x}P_xO$[4]; while in the case of $Ce^{4+}$, $M$ should in principle be vanishingly small since the $4f$-electron becomes itinerant. Therefore, the isothermal magnetization measurement provides an effective indicator for the configuration of the localized electron. In Figure S4a we present isothermal field dependence of magnetization of $CeNiAs_{1-x}P_xO$. All these measurements were performed at 2 K. Linear $M(H)$ dependence far away from saturation was seen in all the P doped samples and no hysteresis could be observed, indicating no obvious ferromagnetic correlation. $M(H)$ doesn't change much with P doping when $x<0.4$, but starts to drop drastically when

$x \geq 0.4$, which is compatible with the behavior of $\chi(T)$. We plot the magnitude of $M$ at 5 T, as well as the Hall coefficient $R_H$ in Figure S4b as a function of P concentration $x$. Similar to the hydrostatic pressure case, $R_H(x)$ jumps from being negative for $x<x_c$ to being positive for $x>x_c$ through an enormous anomaly near $x_c$=0.4. It is evident that the drop of magnetization around $x$=0.4 is accompanied by the change in FS topology, which is consistent with Ce-4$f$ electron's delocalization picture. The magnitude of $R_H$ in the whole doping range is comparable with that in the hydrostatic pressure case, except at the point of $x_c$=0.4. $R_H$ at $x_c$=0.4 shows large positive magnitude, and is one order larger than those of the remaining P doping concentrations. Such a difference is reproducible but is hard to be explained by the single band theory; however, this anomaly does suggest that an unusual Fermi surface (FS) topology transformation is taking place when the QCP is approached.

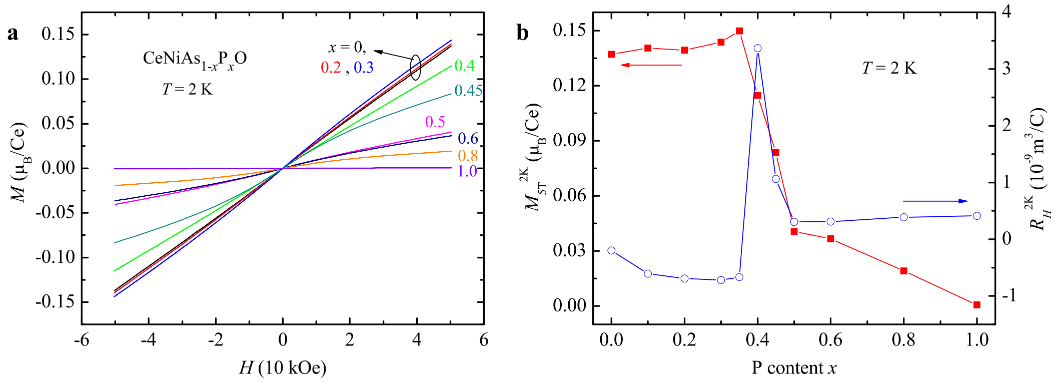


**Figure S4 | Isothermal magnetization of $CeNiAs_{1-x}P_xO$ measured at 2 K. a**, $M(H)$ curves of $CeNiAs_{1-x}P_xO$ measured at 2 K. All the $M(H)$ curves are nearly linear with external field. $M(H)$ doesn't change much with P doping when $x<0.4$, but starts to drop quickly when $x \geq 0.4$. The magnitude of magnetization at 5 T was shown in **b**, together with Hall coefficient $R_H$ at 2 K.

## *SI V: Theoretical calculations on CeNiAsO and CeNiPO*

For first-principles calculations of the electronic structure of the CeNiAsO and CeNiPO compounds, we have employed the local density approximation + dynamical mean-field theory (LDA+DMFT) approach [6] in the charge self-consistent implementations of Refs. [7, 8], which is based on the full-potential augemented plain-wave Wien2K package [9]. This approach allows taking into considerations local correlation effects that are crucial for the proper description of the strongly-interacting Ce-4$f$ states. Wannier Ce-4$f$ orbitals have been constructed using Kohn-Sham eigenstates within the energy range from -8.2 to 4 eV relative to the Fermi energy. For the on-site Coulomb repulsion we employed the spherical approximation within which the interaction vertex is fully specified by the values of the average repulsion $U$ (or the Slatter $F_0$ parameter) and the Hund's rule coupling $J$. The value $U$=7.54 eV has been obtained using a constrain LDA approach. The value of $J$ in rare-earth ions is known to be insensitive to the crystalline environment; we used $J$=0.7 eV obtained from extrapolation of the data from Ref. [10].

In order to solve the DMFT quantum impurity problem we have employed the numerically-exact hybridization-expansion continuous-time quantum Monte-Carlo (CTQMC)[11] method, which allowed us to directly calculate heavy-fermion phases. These calculations were performed for the range of temperatures down to $T$=12 K and with the density-density approximation for the interaction vertex. The spin-orbit and crystalline field splittings were taken into account. We employed the basis of atomic eigenstates (computed neglecting the hybridization function) for the 4$f$ shell occupancy $n$=1 in the quantum impurity problem. In this basis the level positions are diagonal, and we neglected small off-diagonal matrix elements of the 4$f$ hybridization function to make the CTQMC calculations feasible. We used $10^{11}$ CTQMC moves to solve the impurity problem with measurements performed after each 200 moves. A stochastic maximum entropy method was employed for analytical continuation of the self-energy to the real-energy axis. This self-energy was then used to compute the LDA+DMFT density of states and Fermi surfaces.

We have also estimated the single-impurity Kondo scale $T_K$ using a simpler two-step approach. First, we performed LDA+DMFT calculations for the local moment phase of CeNiAs(P)O employing the Hubbard-I approximation[12] to solve the quantum impurity problem. Then the obtained values of the 4$f$ level position [-2.77 (-2.40) eV for CeNiAs(P)O,

respectively], crystalline field and spin-orbit splittings and frequency-dependent hybridization function were used in Gunnarsson-Schönhammer variational calculations of $T_K$[13].

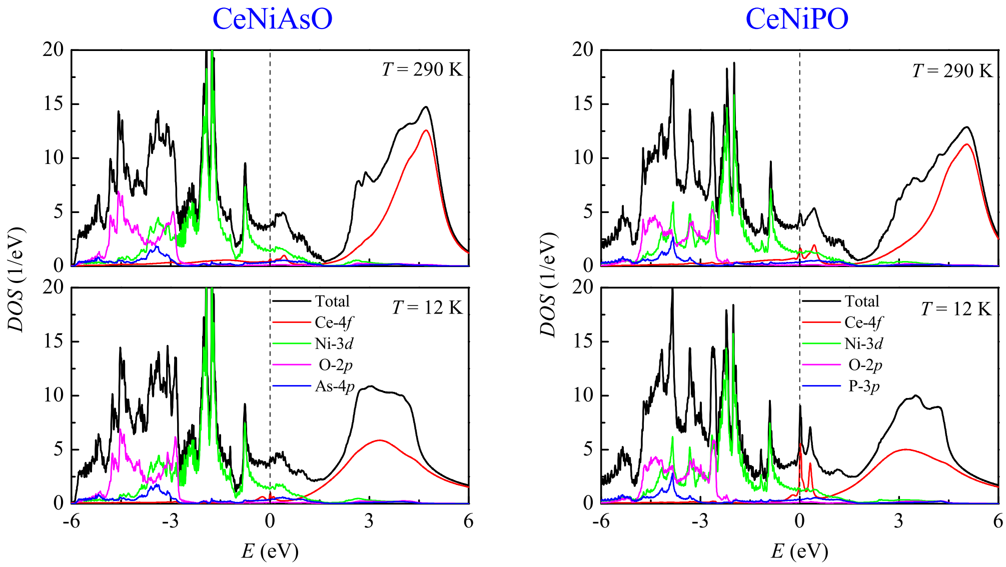


**Figure S5 | The calculated LDA+DMFT density of states (*DOS*) of CeNiAsO (left) and CeNiPO (right)** for temperatures of 290 K (top) and 12 K (bottom), respectively. The total and partial Ce-4$f$, Ni-3$d$, O-2$p$ and As-4$p$ (or P-3$p$) *DOS* are shown in black, red, green, magenta, and blue, respectively. The Kondo peak at $E_F$ formed by renormalized 4$f$ bands, as well as its spin-orbit satellite located at 0.4 eV above $E_F$, are clearly seen in the CeNiPO *DOS* already at $T$=290 K, and their spectral weight is substantially increased at $T$=12 K. *DOS* of CeNiAsO exhibit almost no changes with temperature, with the Ce-4$f$ shell remaining in the local moment regime with almost no Ce-4$f$ spectral weight at the Fermi level.

The density of states (*DOS*) of both compounds calculated by the LDA+DMFT approach in conjunction with the CTQMC method are shown in Figure S5. A Kondo peak formed by renormalized Ce-4$f$ states (which contribution to the *DOS* is shown by the red line in Figure S5) is observed in CeNiPO in the vicinity of the Fermi level $E_F$ already at $T$=290 K. Its spectral weight is clearly increased at low temperature of 12 K indicating that the formation of heavy-fermion band is not completed at room temperature. In contrast, no Kondo peak is observed in CeNiAsO even at $T$=12 K. The remarkable difference between

CeNiAsO and CeNiPO is due to a stronger $3d$-$4f$ hybridization and $4f$ level position being closer to the Fermi level in the latter. This difference leads to a much larger value for the single-impurity Kondo scales in CeNiPO, $T_K$=527 K, compared to $T_K$=15 K in CeNiAsO as obtained by the variational approach[13]. Such drastic increase of $T_K$ from CeNiAsO to CeNiPO also supports the obvious pressure effect on the physical properties of CeNiAsO, and is compatible with the rapidly increasing $T_0$ with pressure.

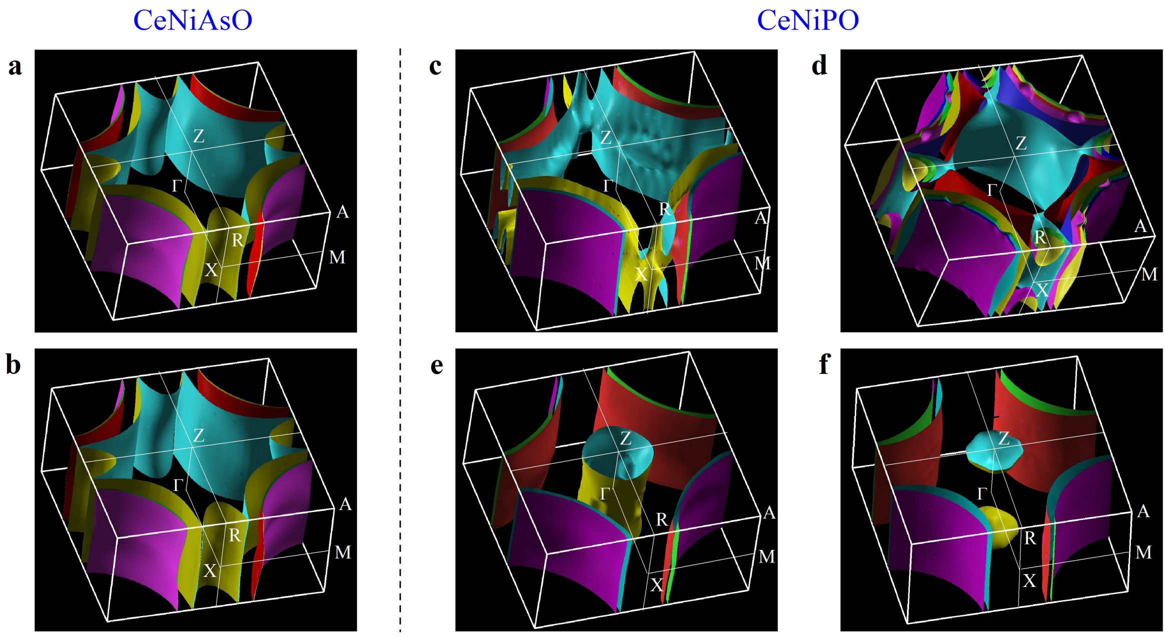


**Figure S6 | The calculated Fermi surfaces (FS) of CeNiAsO and CeNiPO as functions of temperature**. **a-b**, The LDA+DMFT Fermi surfaces of CeNiAsO for temperatures of 290 K (**a**) and 12 K (**b**). One may notice that the FS shape of CeNiAsO is not affected by lowering of temperature and always consists of 2D Fermi sheets. **c-f** The LDA+DMFT Fermi surfaces of CeNiPO for temperatues of 1160 K (**c**), 290 K (**d**), 58 K (**e**), and 12 K (**f**). With lowering temperature the outer quasi-2D FS sheets centered at $M$-$A$ and $X$-$R$ lines first merge into a single cylindrical sheet centered at the $\Gamma$-$Z$ line. At lower temperature this sheet in turn transforms into a single 3D hole pocket around $Z$ point.

We have also employed the same LDA+DMFT+CTQMC approach to calculate the FS topology of CeNiAsO and CeNiPO as a function of temperature, which are shown in Figure S6. The FS of CeNiAsO (Figure S6a-b) is very similar to that of LaNiAsO[5] and exhibits almost no changes with lowering temperature. This FS consists of four sheets: three big electron-like cylinders (two of which are very close to each other) centered at the $M$-$A$ path, and one small hole-like cylinder around $X$-$R$ line. All the FS sheets disperse very weakly along $k_z$ direction, indicating their two-dimensional (2D) character.

In contrast, the FS of CeNiPO is drastically modified by temperature due to a gradual formation of the heavy-electron Ce-4$f$ band in the vicinity of its Fermi level. First, the outer 2D sheet becomes more dispersive along $k_z$ axis even at the highest temperature of 1160 K that we have considered. At lower temperature of $T$=290 K these sheets and the cylinder around the $X$-$R$ line transform into a cylinder-like structure along the $\Gamma$-$Z$ line and small dumbbell-like pockets form around the $R$ point. Further lowering of temperature leads to disappearance of these small pockets and to a progressive narrowing of the cylinder-like sheet (Figure S6e), which at yet lower $T$ transforms into a 3D hole pocket centered at the $Z$ point (Figure S6f). This pocket could be responsible for the sign change in Hall coefficient at the QCP. One should also notice that the total number of electrons enclosed by FS has been significantly enlarged from CeNiAsO to CeNiPO, which is a consequence of participation into the $DOS$ of Ce-4$f$ electrons.

---


[1] Huntelaar, M. E., Booij, A. S., Cordfunke, E. H. P., & van der Laan R. R. The thermodynamic properties of $Ce_2O_3$(s) from $T\rightarrow 0$ K to 1500 K. *J. Chem. Thermodynamics* **32**, 465-482 (2000).

[2] Izumi, F., & Ikeda, T. A Rietveld-Analysis Programm RIETAN-98 and its Applications to Zeolites. *Mater. Sci. Forum* **198**, 321-205 (2000).

[3] Jesche, A., Krellner, C., Souza, M. de, Lang, M. & Gelbel, C. Rare earth magnetism in CeFeAsO: a single crystal study. *New J. Phys.* **11**, 103050 (2009).

[4] Luo, Y. *et al.* Phase diagram of $CeFeAs_{1-x}P_xO$ obtained from electrical resistivity, magnetization, and specific heat measurements. *Phys. Rev. B* **81**, 134422 (2010).

[5] Xu, G. *et al.* Doping-dependent Phase Diagram of LaO$M$As ($M$=V-Cu) and Electron-type

Superconductivity near Ferromagnetic Instability. *EPL* **82**, 67002 (2008).

[6] Kotliar, G. *et al.* Electronic structure calculations with dynamical mean-field theory. *Rev. Mod. Phys.* **78**, 865-951 (2006).

[7] Aichhorn, M. *et al.* Dynamical mean-field theory within an augmented plane-wave framework: Assessing electronic correlations in the iron pnictide LaFeAsO. *Phys. Rev. B* **80**, 085101 (2009).

[8] Aichhorn, M., Pourovskii, L. & Georges, A. Importance of electronic correlations for structural and magnetic properties of the iron pnictide superconductor LaFeAsO. *Phys. Rev. B* **84**, 054529 (2011).

[9] Blaha, P., Schwarz, K., Madsen, G., Kvasnicka, D. & Luitz, J. *WIEN2k, An augmented Plane Wave + Local Orbitals Program for Calculating Crystal Properties.* (Techn. Universitat Wien, Austria, 2001).

[10] Carnall, W. T., Goodman, G. L., Rajnak, K., & Rana, R. S. A systematic analysis of the spectra of the lanthanides doped into single crystal $LaF_3$. *J. Chem. Phys.* **90**, 3443-3457 (1989).

[11] Gull, E. *et al.* Continuous-time Monte Carlo methods for quantum impurity models, *Rev. Mod. Phys.* **83**, 349-404 (2011).

[12] Hubbard, J. Electron Correlations in Narrow Energy Bands. *Proc. Roy. Soc. (London)* **A 276**, 238-257 (1963).

[13] Gunnarsson, O. & Schönhammer, K. Electron spectroscopies for Ce compounds in the impurity model. *Phys. Rev. B* **28**, 4315-4341 (1983).
